# Supplementary material for: Omnia de EgoTempo: Benchmarking Temporal Understanding of Multi-Modal LLMs in Egocentric Videos
Source: arXiv:2503.13646 source file (2025-03-17)
Supplement: Supplementary file 1 [file supplementary.tex]

% CVPR 2025 Paper Template; see https://github.com/cvpr-org/author-kit

\documentclass[10pt,twocolumn,letterpaper]{article}

%%%%%%%%% PAPER TYPE  - PLEASE UPDATE FOR FINAL VERSION
\usepackage{cvpr}              % To produce the CAMERA-READY version
% \usepackage[pagenumbers]{cvpr} % To force page numbers, e.g. for an arXiv version

% Import additional packages in the preamble file, before hyperref
%
% --- inline annotations
%

% --- disable by uncommenting  
% \renewcommand{\TODO}[1]{}
% \renewcommand{\todo}[1]{#1}

\usepackage{amssymb}
\usepackage{amssymb}% http://ctan.org/pkg/amssymb
\usepackage{pifont}% http://ctan.org/pkg/pifont

\usepackage{graphicx}
\usepackage{subcaption}
\usepackage{adjustbox}
\usepackage{colortbl}
\usepackage{longtable}
\usepackage[table,xcdraw]{xcolor}

\usepackage{multirow}
\usepackage{array}
% It is strongly recommended to use hyperref, especially for the review version.
% hyperref with option pagebackref eases the reviewers' job.
% Please disable hyperref *only* if you encounter grave issues, 
% e.g. with the file validation for the camera-ready version.
%
% If you comment hyperref and then uncomment it, you should delete *.aux before re-running LaTeX.
% (Or just hit 'q' on the first LaTeX run, let it finish, and you should be clear).
\definecolor{cvprblue}{rgb}{0.21,0.49,0.74}
\usepackage[pagebackref,breaklinks,colorlinks,allcolors=cvprblue]{hyperref}
\usepackage[table]{xcolor} % for coloring cells
\usepackage{xcolor} % for text color
\usepackage{comment}
\usepackage{subcaption}
\makeatletter
\apptocmd{\@maketitle}{\centering\insertfig}{}{}% insert the figure after authors

%%%%%%%%% PAPER ID  - PLEASE UPDATE
 % *** Enter the Paper ID here

%%%%%%%%% TITLE - PLEASE UPDATE
%\title{\textit{EgoTempo}: Benchmarking Temporal Understanding \\of Multi-Modal LLMs in Egocentric Videos}
\title{\textit{Omnia de} Ego\textit{Tempo}: Benchmarking Temporal Understanding \\of Multi-Modal LLMs in Egocentric Videos}
%\title{In Search of Lost Temporal Understanding: \\Benchmarking Multi-Modal LLMs on Egocentric Videos}

%%%%%%%%% AUTHORS - PLEASE UPDATE
\author{First Author\\
Institution1\\
Institution1 address\\
{\tt\small firstauthor@i1.org}
% For a paper whose authors are all at the same institution,
% omit the following lines up until the closing ``}''.
% Additional authors and addresses can be added with ``\and'',
% just like the second author.
% To save space, use either the email address or home page, not both
\and
Second Author\\
Institution2\\
First line of institution2 address\\
{\tt\small secondauthor@i2.org}
}

\makeatletter

\begin{document}
%\maketitle
\input{sec/X_suppl}    
{
    \small
    \bibliographystyle{ieeenat_fullname}
    \bibliography{main}
}

% WARNING: do not forget to delete the supplementary pages from your submission 
% \input{sec/X_suppl}

\end{document}
